# Supplementary material for: Specification Decomposition for Reactive Synthesis
Source: arXiv:2103.08459 source file (2021-12-16)
Supplement: Supplementary file 1 [file appendix.tex]

\section{Decomposition of LTL Formulas}\label{app:ltl}
